# Supplementary material for: RODEO: Robust Outlier Detection via Exposing Adaptive Out-of-Distribution Samples
Source: arXiv:2501.16971 source file (2025-01-28)
Supplement: Supplementary file 1 [file Appendix.tex]

\newpage
      \begin{center}
\maketitle{\huge \textbf{Appendix} }
    \end{center}

\section{Datasets\&Implementation Details}

\paragraph{Datasets:}For the low-resolution datasets, we included CIFAR10\cite{krizhevsky2009learning}, CIFAR100\cite{krizhevsky2009learning}, MNIST\cite{lecun-mnisthandwrittendigit-2010}, and FashionMNIST\cite{xiao2017fashionmnist}. The results are available in Table \ref{Table 1.a:Novelty Detection for Low-Resolution}. Furthermore, we performed experiments on medical and industrial high-resolution datasets, namely Head-CT\cite{felipe-campos-kitamura_2018}, MVTec-ad\cite{bergmann2019mvtec}, Brain-MRI\cite{brainmri}, Covid19\cite{cohen2020covid}, and Tumor Detection\cite{msoud-nickparvar_2021} and reported the results in Table \ref{Table 1.b:Novelty Detection for High-Resolution}. 

\input{Figures/Third_Figure}

 \textbf{Implementation Details}: We use ResNet-18\cite{resnet} as the architecture of our neural network for the high-resolution datasets and for the low-resolution datasets, we used Wide ResNet\cite{zagoruyko2017wide}. Furthermore, RODEO is trained 10 epochs with Adam\cite{kingma2017adam} optimizer with a learning rate of 0.001 for each experiment. Further details of the implementation of experiments can be found in Appendix

  \section{Algorithm}
This algorithm presents the complete approach, including all components that are integral to it.

\scalebox{1}{
    \begin{algorithm}[H] 
        \SetAlgoLined
    		\KwIn{$\mathcal{D}_{\text{in}}$, $enc_{text}$, $\mu_{Glide}$, $\Sigma_{Glide}$, $f_{clip}$, $g_{clip}$, $f_\theta$, $K$, $T_0$, $T$ \tcp*{ $T_0 \in [0.3T, 0.6T]$ } }
    		
            \KwOut{$\hat{f}_{\theta}$} 
            \tcp{Near-Distribution OOD Prompt Search}
            \For{$(i, label) \in Y$}{
                  $Prompts[i] \leftarrow enc_{text}.KNN(label) \cup Append(NegativeAdjectives[label], label)$ \\
                  $Prompts[i] \leftarrow Prompts[i].Filter( enc_{text}.MinDist(Prompt  ,  Y \ \backslash \ label) > \epsilon$ )
            }
            \tcp{Adaptive Exposure Generation}
            \For{$(x_i, y_i) \in \mathcal{D}_{\text{in}}$}{
                          $c \sim \mathcal{U}(Prompts[y_i])$ \\
                          $t_{init} \sim \mathcal{U}([T_0, ..., T]$ \\
                          $\hat{x}_{t_{init}} = x_i$ \\
                          \For{$t=t_{init} , ... , 0$} {
                            $ \hat{\mu}(\hat{x}_t | c) = \mu_{Glide}(\hat{x}_t|c) + s \cdot \Sigma_{Glide}(\hat{x}_t|c)\cdot \nabla_{\hat{x}_t} (f_{clip}(\hat{x}_t) \cdot g_{clip}(c)) $ \\
                            $ \hat{x}_{t-1} \sim \mathcal{N}( \ \hat{\mu}(\hat{x}_t | c) \ , \  \Sigma_{Glide}(\hat{x}_t|c) \ ) $ \\
                          } 
                          $\mathcal{D}_{\text{exposure}} \leftarrow \mathcal{D}_{\text{exposure}} \cup \{ (\hat{x}_0, K+1) \}$
                    }
    
            $\mathcal{D}_{\text{train}} \leftarrow \mathcal{D}_{\text{in}} \cup \mathcal{D}_{\text{exposure}}$ \\
            $ \hat{f}_{\theta} \leftarrow \text{AdversarialTraining}(f_{\theta}, \mathcal{D}_{\text{train}}) $

            \caption{RODEO: Adv. Training with Adaptive Exposure Dataset}
            \label{alg:RODEO}
    \end{algorithm}
}

\section{Theory and Illustration for Deeper Insight.}
\begin{figure}[h]
  \begin{center}
    \includegraphics[width=1\linewidth]{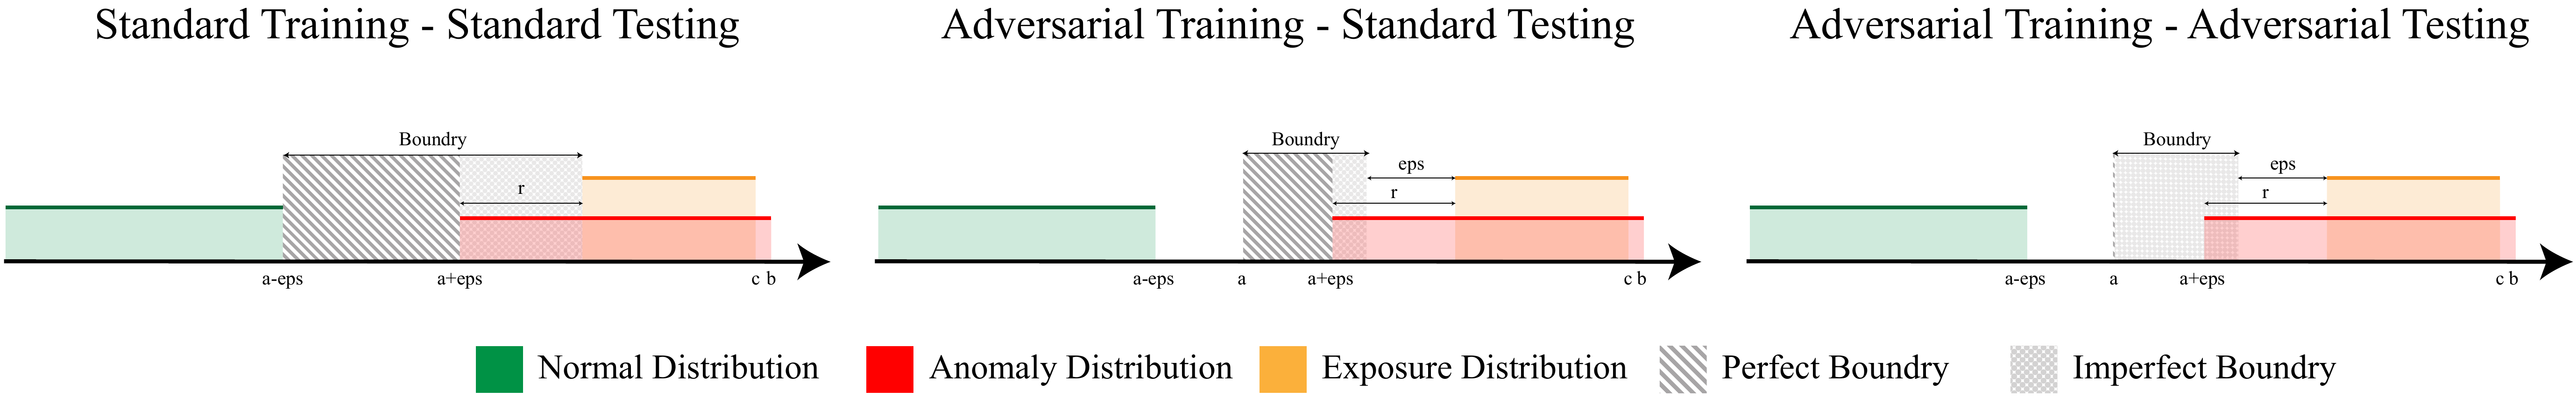}
 %    \caption{Illustration of an insightful example in a one-dimensional feature space, where the outlier 
 % exposure distribution is a subset of the true outliers. The set of feasible thresholds that separate the training data perfectly (green, which is normal, and orange, which is the outlier exposure set) are gray colored. $r$ represents the amount of shift in exposed outliers with respect to the actual anomaly distribution. The subset of feasible values that lead to a perfect test AUROC are bold grays.
 % \\
 %  \textbf{Left}: The standard training and testing scenario. Perfect thresholds constitute a significant proportion of feasible values, even when the outlier exposure are located far from normal samples. 
 % \\
 % \textbf{Middle}: Using adversarial training, the set of feasible thresholds  reduces significantly due to the nature of maximum margin of adversarial training. This in turn reduces the set of perfect thresholds. A large deviation of outlier exposure samples from the actual anomaly distribution lead to a small set of perfect thresholds relative to the set of feasible thresholds. 
 % \\
 %  \textbf{Right}: In the case of adversarial testing, the overlap between the set of feasible and perfect thresholds shrinks to a single point $a$. This shows that the near-distribution property of the exposed outliers is more critical in the adversarial setting as it shrinks the relative size of the set of perfect solutions with respect to the feasible ones. }
     \caption{Effect of the outlier exposure distribution in a one-dimensional feature space in the adversarial and standard setups. Gray regions indicate feasible thresholds for separating the classes in the training data, where green represents the normal class and orange represents the outlier exposure. The parameter \(r\) measures the shift in exposed outliers relative to the actual anomalies, and bold grays indicate thresholds yielding perfect test AUROC values. \textbf{Left:} Standard training scenario with many perfect thresholds, even with distant outlier exposure. \textbf{Middle:} Adversarial training narrows the set of perfect thresholds by reducing the feasible options. \textbf{Right:} During adversarial testing, the set of perfect thresholds contracts to a single point \(a\), highlighting the criticality of near-distribution exposure in adversarial setups.}

    \label{fig:Comparison_Plot}
  \end{center}
\end{figure}

  \section{ND, OSR and OOD Detection} \ 
  
As we have reported the results of our method on the most common settings for OOD detection, in this section, we provide a brief explanation for each setting to provide further clarification.
  In OSR, a model is trained on $K$ classes from an $N$-class training dataset. During testing, the model encounters $N$ distinct classes, where $N-K$ of these classes were not present during the training phase. ND is a type of open-set recognition that is considered an extreme case, specifically when $k$ is equal to 1.
  Some works refer to ND as one-class classification. OOD detection shares similarities with OSR; however, the key distinction is that the open-set and closed-set classes originate from two separate datasets. \cite{yang2021generalized,mirzaei2022fake}

  \section{Details About Evaluation and Generation}

In this section, we will provide more details about our evaluation methodology and Generation Step.
\subsection {Generation Step}

In our proposed generation method, we perturb the ID images with Gaussian noise and utilize GLIDE with guidance from the extracted candidate near OOD labels to shift the ID data to OOD data. This is possible because it has been shown that the reverse process can be solved not only from $t_0=1$ but also from any intermediate time (0, 1). We randomly choose an initial step for each data between 0 and 0.6, which is a common choice based on previous related works. \cite{kim2022diffusionclip,meng2021sdedit}

If we have k classes in the normal dataset, with each class containing N samples, we generate N OOD samples to extend the dataset to k+1 classes. However, if N is a small number (e.g. N<100), we may generate up to 3000 OOD samples to prevent overfitting.

\subsection {PGD Attack on OOD Detectors}

Suppose we have a test dataset containing data samples $\mathrm{x}$ that belong to either the OOD class (-1) or the ID class (1). We can also assume the existence of a trained OOD detector $O_{\boldsymbol{\theta}} : \mathbb{R}^d \rightarrow \mathbb{R}$, which can evaluate an OOD score for each data sample. Depending on the label $\mathrm{y}$, we can generate adversarial examples using the $l_{\infty}$-norm. This involves perturbing the input $l_{\infty}$ in such a way that modifies its OOD score either upwards or downwards:

$$
{x_{0}^*}=x,\ \  \ \  \ \ 
x^{t+1} = x^t + \alpha\cdot \text{sgn}( \nabla_{ x}( y.O_{\boldsymbol{\theta}}(x^t)) )
$$
 
\subsection{Computational Cost}
We conducted our experiments using a single P100 GPU. It takes 2 hour to generate about 10k low-resolution OOD data and near 1k high-resolution OOD data. For each class of low-resolution datasets in one-class classification setting, it takes about 2 hours to train the network and test it. For OOD detection task, it takes about 5 hours to train the network and evaluate the model against all OOD datasets. Each experiment of OSR setting takes about 9 hours of GPU for training and testing as it consists of repeated sampling of ID classes.

\section{Using Image Labels as Descriptors}

Novelty detection, also known as one-class classification, involves identifying instances that do not fit the pattern of a given class in a training set. Traditionally, methods for this task have been proposed without using the labels of the training data. For example, they did not take into account the fact that the normal set includes the semantic "\texttt{dog}". In the case of OOD detection (which is a multi-class setting), methods commonly extract features and define supervised algorithms using the labels of the normal set. However, they do not fully utilize the semantic information contained in these labels. Specifically, they only consider class labels as indexes for their defined task, such as classification.

Recently, there has been a growing interest in leveraging pre-trained multimodal models to enhance OOD detection performance, both in one-class and multi-class scenarios. Unlike prior works, these approaches utilize the semantic information embedded within the labels of the normal set. This is akin to treating labels as image descriptors rather than just as indices. For example, \cite{liznerski2022exposing} used CLIP in the novelty detection setting and utilized both pairs of normal images and their labels (e.g., a photo of {x}) to extract maximum information from the normal set. Similarly, \cite{esmaeilpour2022zero} applied CLIP for zero-shot OOD detection and used both the image and semantic content of their respective labels to achieve the same goal. Motivated by these works, our study utilizes image labels as descriptors in all reported settings (ND, OSR, OOD). In fact, we utilized a simple language model to predict candidate unseen labels for OOD classes located near the boundary, leveraging these image labels.
\paragraph{Discussion} Although some recent works have used labels as descriptors, there may be concerns that this approach could provide unfair guidance since it is not commonly used in traditional literature. However, it is important to note that the OOD detection problem is a line of research with many practical applications in industries such as medicine  autonomous driving cars and industry. In such cases, knowing the training data labels and semantics, such as \textit{"healthy CT scan images"}, is possible and we do not need more details about normal data classes except for their names.

 Moreover, previous adversarially robust OOD detector models have reported almost no improvement over random results in real-world datasets, especially in the case of ND settings. Therefore, our use of the normal class label as an alternative solution is reasonable. Our approach outperforms previous models by up to 50\% in the robust ND scenario and this superiority continues in multi-class modes where data labels are available and we only use the class names to improve the model. Given the applicability of the task addressed in this article and the progress of multi-domain models, our approach has potential for practical use

  \section{Leveraging Pre-trained Models for OOD Detection}
It has been demonstrated that leveraging pre-trained models can significantly improve the performance and practical applicability of downstream tasks \cite{wei2021pretrained,wang2022bridging}, including OOD detection, which has been extensively studied. 

Various works \cite{bergman2020deep,reiss2021panda,reiss2021mean,cohen2021transformaly,roth2021total,Salehi_2021_CVPR} have utilized pre-trained models' features or transfer learning techniques to improve detection results and efficiency, particularly in OOD detection under harder constraints. For example, \cite{esmaeilpour2022zero} used a pre-trained CLIP model trained on 400 million data for Zero-Shot OOD Detection, \cite{fort2021exploring} proposed using a pre-trained ViT \cite{dosovitskiy2020image} model trained on 22 million data for near-OOD detection, and \cite{xu2021unsupervised} utilized a pre-trained BERT \cite{devlin2018bert} model trained on billions of data for OOD detection in the text domain. In our work, we addressed the highly challenging task of developing an adversarially robust OOD detector model, which is unexplored for real-world datasets such as medical datasets. To accomplish this, we utilized the GLIDE model as our generator backbone, which was trained on 67 million data.

  \section{Why GLIDE is the Best Fit for Our Pipeline?}
 
GLIDE, which stands for "Guided Language-to-Image Diffusion for Generation and Editing," is a model developed by \cite{nichol2021glide} that uses diffusion-based text-conditional image synthesis to create images from text prompts. The model combines a diffusion model with CLIP embedding conditioning to generate high-quality images that are photorealistic and can be edited through natural language. 
In the following sections, we will analyze why GLIDE is better suited than other models for generating diverse and near-distribution OOD data.
 \paragraph{Training Time Sample Complexity}
In this work, we utilized GLIDE as our generator backbone to shift the training samples from in-distribution to out-of-distribution. To achieve this, we conditioned GLIDE on images and extracted text from in-distribution sample labels. This leveraging helped us to sample near distribution OODs. Among state-of-the-art text-to-image-based diffusion models, GLIDE stands out because it can generate good samples with a relatively small amount of data. Specifically, the GLIDE model we used in our pipeline, along with its CLIP model, was trained on only \textbf{67 million} text-image pairs, which is much smaller than the common data amount that text-to-image models are typically trained on, which is in the \textbf{Billion-scale}. For example, the Stable Diffusion model was trained on the LAION-5Billion \cite{schuhmann2022laion} dataset.

 \paragraph{GLIDE Works in Pixel Space    }
In Section \ref{two_type_ood}, we discussed how OOD data can be divided into two categories (i.e. pixel- and semantic-level). Our need for diverse OOD data motivates our preference for generative models that can create both pixel-level and semantic-level OOD data. GLIDE is a suitable choice as it uses a diffusion model applied at the pixel-level to generate images from natural language prompts. This allows GLIDE to generate OOD samples that differ in their local appearance, which is particularly important for pixel-level OOD detection. Compared to other state-of-the-art text-to-image models that mostly work at the embedding level, GLIDE's ability to generate images at the pixel-level makes it a better choice for our purposes.
 \paragraph{Comparing GLIDE with DreamBooth}
As our pipeline's generator model involves image editing, we explored the literature on image manipulating and tested a common methods used for image editing. Numerous algorithms have been proposed for generating new images conditioned on input images  among these, we have chosen DreamBooth as one of the SOTA algorithms for specifying image details in text-to-image models.  we evaluated the DreamBooth algorithm for changing image details in various datasets. Our experiment showed that, despite DreamBooth's good performance for natural images and human faces, the algorithm had poor results for datasets with different distributions, such as MNIST and FashionMNIST. One possible explanation for the poor performance of these algorithms is their bias towards the distribution of the training datasets, such as LAION, which typically consists of natural images and portraits. Consequently, these algorithms may not yield satisfactory results for datasets with different distributions.

\input{Figures/Stable-Diffusion}

\section{Detailed Analysis and Insights of Ablation Study}
In this section, we provide additional details about our ablation study, including our evaluation setting and metrics. As shown in Table \ref{Table:Ablation_1}, we reported our results in the ND setting, where each entry corresponds to a specific target dataset (e.g. MNIST) and a source of outlier exposure (e.g. CIFAR10).

For example, in the MNIST \& CIFAR10 case, we treated one class of MNIST (e.g. digit 0) as our normal set, and the remaining classes (e.g. digits 1 to 9) as OOD data that our model had to detect during testing. We used the CIFAR10 dataset as our source of outlier exposure and trained our binary classifier adversarially to classify both the normal class of MNIST and the OOD data from CIFAR10.

Since we were working in the Novelty Detection setting, we repeated this process for each class of the targeted dataset and reported the mean of the results (e.g. average of 10 results for the MNIST case) in the corresponding table entry.

It's worth noting that the diagonal of the table (e.g., MNIST\&MNIST) indicates that the targeted dataset and exposed dataset are the same. For example, in the MNIST\&MNIST case, we considered one class of MNIST (e.g., digit 0) as the normal set, while the remaining classes (e.g., digits 1 to 9) were considered as OOD data. We then randomly dropped a subset of the OOD data and used the dropped data as the outlier exposure during training. In these cases, the distribution of the normal set and the exposed dataset has a lower distance between them. Consequently, the superiority of the results in the diagonal compared to other entries indicates that utilizing a near-distribution outlier exposure can improve the adversarial robustness of the model.

In Table \ref{Table:Ablation_2}, we aimed to demonstrate the importance of both the diversity of the generated OOD data and the distance between the distribution of the exposed outliers and the normal data. To measure this distance, we used the Fréchet Inception Distance (FID) metric to compare the generated data in our proposed pipeline with the normal data. Our results indicate that, overall, the generated OOD data in our pipeline has a lower distance to the normal data compared to other datasets/OE techniques. Additionally, we achieved better diversity, as evidenced by the Density and Coverage metrics.

In the following, we will provide more details about the Fréchet Inception Distance (FID) and Density\&Coverage metrics.

\paragraph{Density \& Coverage and FID }\label{DENSITY}
FID measures the distance between feature vectors of real and generated images and calculates the distance them, has been shown to match with human judgments.

{\color{black} The diversity of generative models can be evaluated using two metrics: Density and Coverage \cite{naeem2020reliable}. By utilizing a manifold estimation procedure code, the distance between two sets of images can be measured. To calculate these metrics, features from a pre-trained model are utilized, specifically those before the final classification layer. The mathematical expression for these metrics is as follows}:

\begin{equation} \label{eq_}
    \centering
    \begin{split}
Density\left(\boldsymbol{X}_s, \boldsymbol{X}_t, F, k\right)=\frac{1}{k M} \sum_{j=1}^M \sum_{i=1}^N \mathbb{I}\left(\boldsymbol{f}_{t, j} \in B\left(\boldsymbol{f}_{s, i}, \mathrm{NN}_k\left(F\left(\boldsymbol{X}_s\right), \boldsymbol{f}_{s, i}, k\right)\right)\right) \text {, }
    \end{split}
\end{equation}

\begin{equation} \label{eq_}
    \centering
    \begin{split}
Coverage\left(\boldsymbol{X}_s, \boldsymbol{X}_t, F, k\right)=\frac{1}{N} \sum_{i=1}^N \mathbb{I}\left(\exists j \text { s.t. } \boldsymbol{f}_{t, j} \in B\left(\boldsymbol{f}_{s, i}, \mathrm{NN}_k\left(F\left(\boldsymbol{X}_s\right), \boldsymbol{f}_{s, i}, k\right)\right)\right).
    \end{split}
\end{equation}
 
where $\boldsymbol{F}$ is a feature extractor, $\boldsymbol{f}$ is a collection of features from ${F}$, 

 $\boldsymbol{X}_s=\left\{\boldsymbol{x}_{s, 1}, \ldots, \boldsymbol{x}_{s, N}\right\}$ denotes real images, $\boldsymbol{X}_t=\left\{\boldsymbol{x}_{t, 1}, \ldots, \boldsymbol{x}_{t, M}\right\}$ denotes  generated images , $B(\boldsymbol{f}, r)$ is the $\mathrm{n}$-dimensional sphere in which $\boldsymbol{f}=F(\boldsymbol{x}) \in \mathbb{R}^n$ is the center and $r$ is the radius, $\mathrm{NN}_kf({F}, \boldsymbol{f}, k)$ is the distance from $\boldsymbol{f}$ to the $k$-th nearest embedding in ${F}$, and $\mathbb{I}(\cdot)$ is a indicator function. We use the standard InceptionV3 features, which are also used to compute the FID. The measures are computed using the official code \cite{naeem2020reliable}.

\paragraph{More Details }

We computed the correlation between the diversity and nearness of out-of-distribution (OOD) data, and the robustness of the detector models. The results showed a stronger correlation in adversarial settings compared to clean settings.
\begin{figure}[t]
  \begin{center}
    \includegraphics[width=1\linewidth]{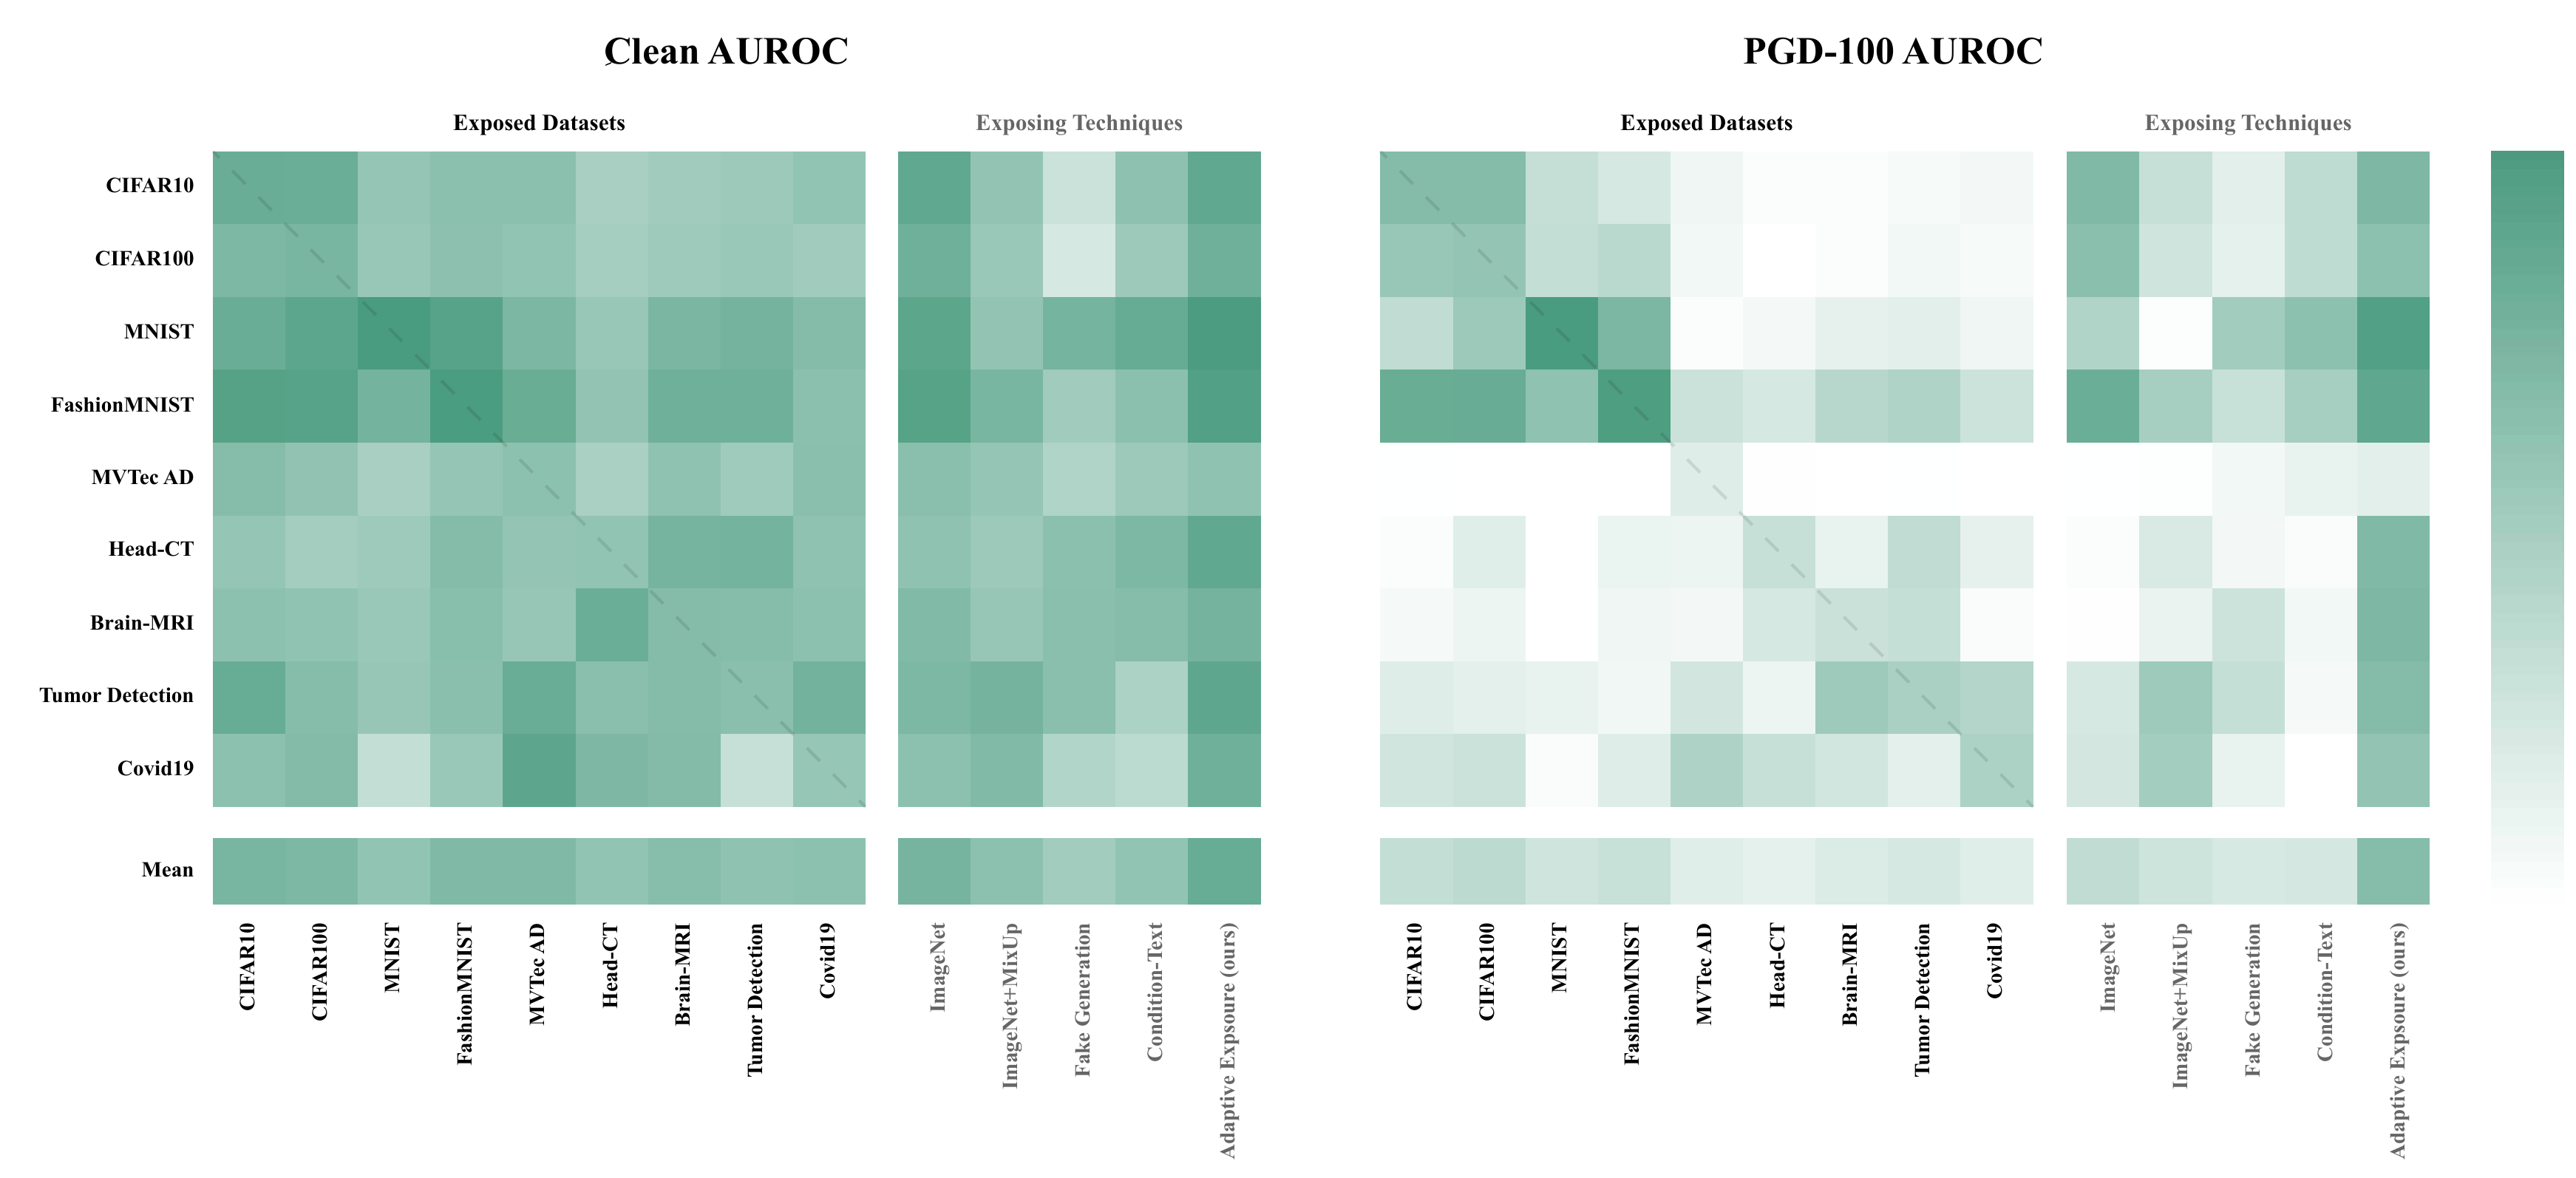}
    \caption{The results demonstrate that when the targeted dataset and the exposed dataset have a smaller distance (as shown on the diagonal), the robustness results are better.}
    \label{fig:Comparison_Plot}
  \end{center}
\end{figure}

\[
NDC=\frac{{\log(density\_values) + \log(coverage\_values)}}{{\log(fid\_values)}}
\]

\begin{table}[h]
\centering
\caption{Correlation between NDC and Detector Performance }
\medskip
\begin{tabular}{|c|c|}
\hline
\textbf{Attack} & \textbf{Correlation} \\
\hline
Clean & 0.280 \\
PGD-100 & 0.448 \\
AutoAttack & 0.460 \\
\hline
\end{tabular}
\end{table}

\section{The Significance of Conditioning on Both Images and Text from the Normal Distribution}

To perform adversarial OOD data, it's important to generate diverse and realistic samples that are close to the distribution of the normal data. In our study, we tackle this challenge by leveraging the information contained in the normal data. Specifically, we extract the labels of classes that are close to the normal set and use them as guidance for generation. Additionally, we initialize the reverse process generation of GLIDE with normal images, so the generation of OOD data in our pipeline is conditioned on both the images and the text of the normal set. This enables us to generate adaptive OOD samples.

In the Ablation Study section \ref{Ablation_Section}, we demonstrate the importance of using both image and text information for generating OOD data. We compare our approach with two other methods that condition on only one type of information and ignore the other. The first technique generates fake images based on the normal set, while the other generates OOD data using only the extracted text from normal labels. The results show that both techniques are less effective than our adaptive exposure technique, which conditions generation on both text and image. This confirms that using both sources of information is mandatory and highly beneficial. Specifically, In Table 3-a\ref{Table:Ablation_1}, the 'Condition-text' column shows the results when generating OOD data using only the extracted text from normal labels as prompts via GLIDE, while the 'Fake generation' column shows the results when generating OOD data by conditioning on normal images alone. Specifically, the 'Fake generation' technique \cite{mirzaei2022fake} refers to the proposed method of generating OE using a diffusion model that relies solely on the normal set images. Our adaptive exposure technique achieves superior performance, indicating that conditioning on both text and images is crucial for generating high-quality OOD data.

\subsection{Samples Generated Solely Based on Text Conditioning} 
  In this section, we compare normal images with images generated by GLIDE using only text prompts in figure \ref{fig:Samples_Plot1}  (without conditioning on the images). Our results, illustrated by the plotted samples, demonstrate that there is a significant difference in distribution between these generated images and normal images. This difference is likely the reason for the ineffectiveness of the OOD samples generated with this technique.
\section{Prompt Generation}
  \subsection{Pixel-Level and Semantic-Level OOD Detection}\label{two_type_ood}
OOD samples can be categorized into two types: pixel-level and semantic-level. In pixel-level OOD detection, ID and OOD samples differ in their local appearance, while remaining semantically identical. For instance, a broken glass could be considered an OOD sample compared to an intact glass due to its different local appearance. In contrast, semantic-level OOD samples differ at the semantic level, meaning that they have different meanings or concepts than the ID samples. For example, a cat is an OOD sample when we consider dog semantics as ID because they represent different concepts.

\subsection{Our Method of Generating Prompt} A reliable and generalized approach for anomaly detection must have the capability to detect both semantic-level and pixel-wise anomalies, as demonstrated in section \ref{two_type_ood}. To this end, our proposed method constructs prompts by combining two sets of words: near-distribution prompts and negative adjectives derived from a normal label name. We hypothesize that the former set can detect semantic-level anomalies, while the latter set is effective in detecting pixel-wise anomalies. Additionally, we include an extra prompt, marked as 'others', in the prompts list to augment the diversity of exposures.

To generate negative adjectives, we employ a set of constant prompts that are listed below and used across all experimental settings (X is the normal label name):
    \begin{itemize}
        \item A photo of X with a crack 
        \item A photo of a broken X
        \item A photo of X with a defect 
        \item A photo of X with damage
        \item A photo of X with a scratch 
        \item A photo of X with a hole 
        \item A photo of X torn
        \item A photo of X cut
        \item A photo of X with contamination
        \item A photo of X with a fracture
        \item A photo of a damaged X
        \item A photo of a fractured X
        \item A photo of X with destruction
        \item A photo of X with a mark
    \end{itemize}

For near-distribution prompts, we utilize Word2Vec to search for semantically meaningful word embeddings after normalizing the words through a process of lemmatization. First, we obtain the embedding of the normal class label and then search among the corpus to identify the 1000 nearest neighbors of the normal class label. We then sample prompts from the obtained words based on the similarity factor of the neighbors to the normal class label. The selection probability of the prompts is proportional to their similarity to the normal class label. Finally, we compile a list of prompts to serve as inputs for Glide, which generates adaptive exposures.

\begin{table*}[h ]
\caption{The detailed AUROC scores of the class-specific experiments for (One-Class) Novelty Detection setting in CIFAR10, CIFAR100, MNIST, Fashion-MNIST datasets.}
\label{}
\begin{subtable}{1\textwidth}
\BlankLine
\subcaption{ CIFAR10 }
\label{}
\resizebox{\linewidth}{!}{\begin{tabular}{llr*{13}{c}} 
\hline\noalign{\smallskip}

% The AUROC of various novelty detector models is utilized to evaluate their performance under different attacks. A clean evaluation is conducted on data that is not attacked, while other attacks refer to situations where both normal and abnormal data are attacked. 
  
   \multicolumn{1}{c}{Method} & \multicolumn{1}{c}{Attack} & &\multicolumn{9}{c}{Class } &\multicolumn{1}{c}{ Average }  
     \\      \cmidrule(lr){1-1} \cmidrule(lr){2-2} 
    \cmidrule(lr){3-12}  
    \cmidrule(lr){13-13}   
   
  & &\multirow{2}{*}{0}&\multirow{2}{*}{1}&\multirow{2}{*}{2}&\multirow{2}{*}{3}&\multirow{2}{*}{4} &\multirow{2}{*}{5}&\multirow{2}{*}{6} & \multirow{2}{*}{7} & \multirow{2}{*}{8} &\multirow{2}{*}{9}  \\
  & & & & & &  & &  &   &   & &  \\
  
\noalign{\smallskip}
 \hline

\noalign{\smallskip}
% capsnet: 1911.08616
% rest: ARAE 97.5	\_	64.1	73
\multirow{4}{*}{Ours} &Clean& 91.7 & 97.3 & 77.4 & 74.0 & 82.6 & 81.2 & 91.5 & 92.8 & 94.0 & 91.7 & 87.4
\\ & BlackBox & 89.9 & 95.8 & 75.5 & 72.1 & 81.6 & 79.1 & 89.1 & 91.2 & 92.4 & 89.6 & 85.6
 
\\ & PGD-100& 78.0 & 82.1 & 59.9 & 55.3 & 65.4 & 67.5 & 74.3 & 70.2 & 80.2 & 77.8 & 71.1
 \\ & AutoAttack& 75.7 & 80.0 & 58.7 & 53.6 & 64.2 & 65.1 & 72.1 & 68.8 & 78.9 & 76.0 & 69.3
 
  \\

\noalign{\smallskip}
% capsnet: 1911.08616
% rest: ARAE 97.5	\_	64.1	73

\hline
\end{tabular}}
\end{subtable}

 \bigskip

\begin{subtable}{1\textwidth}
\BlankLine
\subcaption{ CIFAR100 }
\label{}
\resizebox{\linewidth}{!}{\begin{tabular}{llr*{23}{c}} 
\hline\noalign{\smallskip}

% The AUROC of various novelty detector models is utilized to evaluate their performance under different attacks. A clean evaluation is conducted on data that is not attacked, while other attacks refer to situations where both normal and abnormal data are attacked. 
  
   \multicolumn{1}{c}{Method} & \multicolumn{1}{c}{Attack} & &\multicolumn{19}{c}{Class } &\multicolumn{1}{c}{ Average }  
     \\      \cmidrule(lr){1-1} \cmidrule(lr){2-2} 
    \cmidrule(lr){3-22}  
    \cmidrule(lr){23-23}   

  & &\multirow{2}{*}{0}&\multirow{2}{*}{1}&\multirow{2}{*}{2}&\multirow{2}{*}{3}&\multirow{2}{*}{4} &\multirow{2}{*}{5}&\multirow{2}{*}{6} & \multirow{2}{*}{7} & \multirow{2}{*}{8} &\multirow{2}{*}{9} &\multirow{2}{*}{10}&\multirow{2}{*}{11}&\multirow{2}{*}{12}&\multirow{2}{*}{13}&\multirow{2}{*}{14} &\multirow{2}{*}{15}&\multirow{2}{*}{16} & \multirow{2}{*}{17} & \multirow{2}{*}{18} &\multirow{2}{*}{19}  \\

  & & & & & & & & & & & & & & & & & & & & &   \\
  
\noalign{\smallskip}
 \hline

\noalign{\smallskip}
% capsnet: 1911.08616
% rest: ARAE 97.5	\_	64.1	73
\multirow{4}{*}{Ours} &Clean & 79.0 & 78.6 & 95.5 & 78.1 & 89.2 & 69.4 & 76.2 & 82.6 & 77.9 & 87.4 & 92.7 & 73.1 & 77.6 & 65.0 & 83.9 & 65.5 & 72.1 & 93.6 & 83.5 & 72.0 & 79.6
\\ & BlackBox & 76.9 & 77.0 & 93.2 & 75.4 & 87.6 & 67.3 & 74.0 & 79.6 & 75.7 & 85.1 & 89.9 & 71.3 & 74.7 & 62.9 & 81.0 & 63.4 & 69.7 & 91.8 & 81.8 & 70.1 & 77.4
 
\\ & PGD-100 & 59.9 & 61.2 & 83.2 & 62.5 & 74.2 & 53.9 & 61.6 & 63.0 & 59.2 & 76.9 & 78.4 & 51.7 & 61.3 & 49.0 & 61.0 & 45.0 & 54.3 & 79.3 & 61.5 & 59.2 & 62.8
 \\ & AutoAttack & 56.8 & 59.4 & 80.4 & 60.9 & 73.9 & 51.2 & 61.3 & 61.7 & 58.3 & 75.9 & 75.7 & 51.7 & 59.9 & 45.7 & 59.2 & 44.4 & 50.6 & 76.1 & 60.5 & 57.1 & 61.0
 
  \\

\noalign{\smallskip}
% capsnet: 1911.08616
% rest: ARAE 97.5	\_	64.1	73

\hline
\end{tabular}}
\end{subtable}

 \bigskip

\begin{subtable}{1\textwidth}
\BlankLine
\subcaption{ MNIST }
\label{}
\resizebox{\linewidth}{!}{\begin{tabular}{llr*{13}{c}} 
\hline\noalign{\smallskip}

% The AUROC of various novelty detector models is utilized to evaluate their performance under different attacks. A clean evaluation is conducted on data that is not attacked, while other attacks refer to situations where both normal and abnormal data are attacked. 
  
   \multicolumn{1}{c}{Method} & \multicolumn{1}{c}{Attack} & &\multicolumn{9}{c}{Class } &\multicolumn{1}{c}{ Average }  
     \\      \cmidrule(lr){1-1} \cmidrule(lr){2-2} 
    \cmidrule(lr){3-12}  
    \cmidrule(lr){13-13}   
   
  & &\multirow{2}{*}{0}&\multirow{2}{*}{1}&\multirow{2}{*}{2}&\multirow{2}{*}{3}&\multirow{2}{*}{4} &\multirow{2}{*}{5}&\multirow{2}{*}{6} & \multirow{2}{*}{7} & \multirow{2}{*}{8} &\multirow{2}{*}{9}  \\
  & & & & & &  & &  &   &   & &  \\
  
\noalign{\smallskip}
 \hline

\noalign{\smallskip}
% capsnet: 1911.08616
% rest: ARAE 97.5	\_	64.1	73
\multirow{4}{*}{Ours} &Clean & 99.8 & 99.4 & 99.3 & 99.2 & 99.6 & 99.4 & 99.8 & 98.9 & 99.4 & 98.8 & 99.4
\\ & BlackBox & 98.7 & 99.0 & 98.2 & 98.8 & 98.3 & 98.9 & 99.4 & 97.8 & 98.5 & 98.2 & 98.6
 
\\ & PGD-100 & 97.4 & 96.4 & 97.0 & 92.9 & 97.5 & 96.6 & 98.4 & 93.2 & 95.4 & 92.6 & 95.7
 \\ & AutoAttack& 96.9 & 96.1 & 96.3 & 92.0 & 96.7 & 96.3 & 98.1 & 92.5 & 95.2 & 92.0 & 95.2
 
  \\

\noalign{\smallskip}
% capsnet: 1911.08616
% rest: ARAE 97.5	\_	64.1	73

\hline
\end{tabular}}
\end{subtable}

 \bigskip

\begin{subtable}{1\textwidth}
\BlankLine
\subcaption{ Fashion-MNIST }
\label{}
\resizebox{\linewidth}{!}{\begin{tabular}{llr*{13}{c}} 
\hline\noalign{\smallskip}

% The AUROC of various novelty detector models is utilized to evaluate their performance under different attacks. A clean evaluation is conducted on data that is not attacked, while other attacks refer to situations where both normal and abnormal data are attacked. 
  
   \multicolumn{1}{c}{Method} & \multicolumn{1}{c}{Attack} & &\multicolumn{9}{c}{Class } &\multicolumn{1}{c}{ Average }  
     \\      \cmidrule(lr){1-1} \cmidrule(lr){2-2} 
    \cmidrule(lr){3-12}  
    \cmidrule(lr){13-13}   
   
  & &\multirow{2}{*}{0}&\multirow{2}{*}{1}&\multirow{2}{*}{2}&\multirow{2}{*}{3}&\multirow{2}{*}{4} &\multirow{2}{*}{5}&\multirow{2}{*}{6} & \multirow{2}{*}{7} & \multirow{2}{*}{8} &\multirow{2}{*}{9}  \\
  & & & & & &  & &  &   &   & &  \\
  
\noalign{\smallskip}
 \hline

\noalign{\smallskip}
% capsnet: 1911.08616
% rest: ARAE 97.5	\_	64.1	73
\multirow{4}{*}{Ours} &Clean & 95.8 & 99.7 & 93.9 & 93.4 & 92.9 & 98.3 & 86.5 & 98.6 & 98.5 & 98.8 & 95.6
\\ & BlackBox & 94.4 & 98.6 & 92.7 & 92.6 & 91.2 & 96.9 & 85.1 & 97.1 & 97.5 & 97.1 & 94.3
 
\\ & PGD-100 & 90.0 & 98.5 & 83.8 & 81.1 & 77.5 & 95.3 & 72.7 & 95.1 & 92.5 & 94.5 & 88.1
 \\ & AutoAttack & 89.7 & 98.1 & 83.0 & 80.9 & 76.5 & 95.1 & 72.6 & 94.2 & 92.4 & 94.1 & 87.6
 
  \\

\noalign{\smallskip}
% capsnet: 1911.08616
% rest: ARAE 97.5	\_	64.1	73

\hline
\end{tabular}}
\end{subtable}

\end{table*}

\section{OSR Experiments Details}
In order to evaluate earlier works in OSR setting, we first select desired number of classes, say $K$ and rename the labels of samples to be in the range $0$ to $K-1$. Then following the guideline of the method, we evaluate it in both clean and adversarial settings and repeat each experiment 5 times and report the average.

\section{OOD Experiments Details}
Table \ref{Table2.a:OOD} yielded results that are now presented in Table \ref{OOD_details} for a more comprehensive overview. Following the guidelines in Section 4.2, we designated multiple datasets as out-of-distribution during the testing phase and reported the outcomes in Table \ref{OOD_details}. Adversarial and clean out-of-distribution scenarios have also been examined by other approaches. Prominent methods in the clean setting encompass the ViT architecture and OpenGAN. Regarding image classification, AT and HAT have been recognized as highly effective defenses. AOE, ALOE, and OSAD are regarded as state-of-the-art methods for out-of-distribution detection, and ATD in robust OOD detection. These OOD methods (excluding OpenGAN and ATD) have undergone evaluation with various detection techniques, including MSP \cite{hendrycks2017a}\cite{liang2018enhancing}, MD \cite{MD}, Relative MD \cite{ren2021simple}, and OpenMax \cite{openmax}. The results reported for each OOD method correspond to the best performing detection method. Notably, our approach has surpassed the state-of-the-art in robust out-of-distribution setting (ATD) for nearly all datasets.

$$
\mu_k=\frac{1}{N} \sum_{i: y_i=k} z_i, \quad \Sigma=\frac{1}{N} \sum_{k=1}^K \sum_{i: y_i=k}\left(z_i-\mu_k\right)\left(z_i-\mu_k\right)^T, \quad k=1,2, \ldots, K
$$
In addition, to use RMD, one has to fit a $\mathcal{N}\left(\mu_0, \Sigma_0\right)$ to the whole in-distribution. Next, the distances and anomaly score for the input $x^{\prime}$ with pre-logits $z^{\prime}$ are computed as:
$$
\begin{gathered}
M D_k\left(z^{\prime}\right)=\left(z^{\prime}-\mu_k\right)^T \Sigma^{-1}\left(z^{\prime}-\mu_k\right), \quad R M D_k\left(z^{\prime}\right)=M D_k\left(z^{\prime}\right)-M D_0\left(z^{\prime}\right), \\
\operatorname{score}_{M D}\left(x^{\prime}\right)=-\min _k\left\{M D_k\left(z^{\prime}\right)\right\}, \quad \text { score }_{R M D}\left(x^{\prime}\right)=-\min _k\left\{R M D_k\left(z^{\prime}\right)\right\} .
\end{gathered}
$$
 
\begin{table*}[h]
\centering
\caption{OOD detailed results}
\label{OOD_details}
\begin{subtable}{1\textwidth}

\BlankLine
\centering
\subcaption{CIFAR10}
\label{OOD_CIFAR10}
\resizebox{\linewidth}{!}{\begin{tabular}{llr*{9}{c}} 
\hline\noalign{\smallskip}

   \multicolumn{1}{c}{Out-Dataset} & \multicolumn{1}{c}{Attack} &\multicolumn{8}{c}{Method}\\
    \cmidrule(lr){3-10}

  & &OpenGAN&ViT (RMD)& ATOM &AT (OpenMax)&OSAD (OpenMax)& ALOE (MSP)& ATD & RODEO    \\
\noalign{\smallskip}
 \hline
\noalign{\smallskip}
 
\multirow{2}{*}{MNIST}&\multirow{1}{*}{\centering Clean}&\underline{99.4}&\underline{98.7}&98.4&80.4&86.2&74.6&98.8&96.9 \\ &\multirow{1}{*}{\centering PGD-100}&30.3&3.5&0.0&39.6& 55.3&22.7&\textbf{90.2}&\underline{84.0} \\
    \cmidrule(lr){1-1} \cmidrule(lr){2-2} 
    \cmidrule(lr){3-10}

\multirow{2}{*}{TiImgNet}&\multirow{1}{*}{\centering Clean}&\textbf{95.3}&\underline{95.2}&97.2&81.0&81.9& 82.1&88.0&85.1 \\ &\multirow{1}{*}{\centering PGD-100}&15.2&2.3&4.3&16.5&19.3&21.6&\underline{47.0}&\textbf{47.2}  \\
    \cmidrule(lr){1-1} \cmidrule(lr){2-2} 
    \cmidrule(lr){3-10}

\multirow{2}{*}{Places}&\multirow{1}{*}{\centering Clean}&95.0&\textbf{98.3}&98.7&82.5& 83.3& 85.1&92.5&\underline{96.2} \\ &\multirow{1}{*}{\centering PGD-100}&17.3&3.1&6.5&18.9& 21.2  &22.8&\underline{60.7}&\textbf{71.1}  \\
    \cmidrule(lr){1-1} \cmidrule(lr){2-2} 
    \cmidrule(lr){3-10}

\multirow{2}{*}{LSUN}&\multirow{1}{*}{\centering Clean}&96.5 &98.4&99.1&85.0 &   86.4 &  \underline{98.7} &96.0& \textbf{99.0}   \\ &\multirow{1}{*}{\centering PGD-100}&24.0 &2.0 &1.9&19.6 & 20.7  &51.6&\underline{69.0} & \textbf{86.0}  \\
    \cmidrule(lr){1-1} \cmidrule(lr){2-2} 
    \cmidrule(lr){3-10}  

\multirow{2}{*}{iSUN}&\multirow{1}{*}{\centering Clean}&96.3&\textbf{98.6}&99.5&83.9&84.0&\underline{98.3}&94.8&97.7 \\ &\multirow{1}{*}{\centering PGD-100}&23.0&2.1&3.4&19.5&20.3&50.4&\underline{66.8}&\textbf{79.6}  \\
    \cmidrule(lr){1-1} \cmidrule(lr){2-2} 
    \cmidrule(lr){3-10}  

\multirow{2}{*}{Birds}&\multirow{1}{*}{\centering Clean}&\textbf{98.3}&76.0&95.8&75.1&76.5&79.9&93.6&\underline{97.8}\\ &\multirow{1}{*}{\centering PGD-100}&34.5&0.6&6.1&14.7&19.1  &21.8&\underline{69.0}&\textbf{76.9}\\
    \cmidrule(lr){1-1} \cmidrule(lr){2-2} 
    \cmidrule(lr){3-10}  

\multirow{2}{*}{Flower}&\multirow{1}{*}{\centering Clean}&98.3&\underline{99.6}&99.8&85.5&88.6&79.0&\textbf{99.7}&99.5 \\ &\multirow{1}{*}{\centering PGD-100}&30.1&2.6&19.9&20.9&26.6&19.6&\textbf{93.7}&\underline{89.6}\\
    \cmidrule(lr){1-1} \cmidrule(lr){2-2} 
    \cmidrule(lr){3-10}

\multirow{2}{*}{COIL}&\multirow{1}{*}{\centering Clean}&\textbf{98.1}&\underline{95.9}&97.3&70.3&75.0&76.8&90.8&91.1  \\ &\multirow{1}{*}{\centering PGD-100}&38.5&3.9&9.5&16.6&18.7&19.3&\underline{58.1}&\textbf{60.4}\\
    \cmidrule(lr){1-1} \cmidrule(lr){2-2} 
    \cmidrule(lr){3-10}  

\multirow{2}{*}{CIFAR100}&\multirow{1}{*}{\centering Clean}&\underline{95.0}&\textbf{97.3}& 94.2&79.6&79.9&78.8&82.0&75.6\\&\multirow{1}{*}{\centering PGD-100}&10.1&1.70&2.5 &16.0& 18.1 &17.0&\underline{38.0}&\textbf{38.7}\\
    \cmidrule(lr){1-1} \cmidrule(lr){2-2} 
    \cmidrule(lr){3-10}  
 \noalign{\smallskip}
 
\multirow{2}{*}{Avg.}&\multirow{1}{*}{\centering Clean}&\textbf{97.1}&\underline{95.1}& 97.8 &80.5&82.7&84.3&94.3&93.2 \\ &\multirow{1}{*}{\centering PGD-100}&26.6&2.5& 6.0 &20.8&25.1&28.7&\underline{69.3}&\textbf{70.4}\\
 \hline

\end{tabular}}
\end{subtable}

\begin{subtable}{1\textwidth}

\BlankLine
\centering
\subcaption{CIFAR100}
\label{OOD_CIFAR100}
\resizebox{\linewidth}{!}{\begin{tabular}{llr*{9}{c}} 
\hline\noalign{\smallskip}

   \multicolumn{1}{c}{Out-Dataset} & \multicolumn{1}{c}{ Attack}  &\multicolumn{7}{c}{Method}\\
    \cmidrule(lr){3-10}

  & &OpenGAN&ViT (RMD)&ATOM&AT (RMD)&OSAD (MD)& ALOE(MD)& ATD & RODEO    \\
\noalign{\smallskip}
 \hline
\noalign{\smallskip}

\multirow{2}{*}{MNIST}&\multirow{1}{*}{\centering Clean}&\underline{99.0}&83.8&90.4&41.1&95.9&96.6&97.3&\textbf{99.7}&   \\& \multirow{1}{*}{\centering PGD-100}&14.6&1.7&0.0&14.2&82.0&73.1&\underline{86.3}&\textbf{97.7}&  \\
    \cmidrule(lr){1-1} \cmidrule(lr){2-2} 
    \cmidrule(lr){3-10}

\multirow{2}{*}{TiImgNet}&\multirow{1}{*}{\centering Clean}&\underline{88.3}&\textbf{90.1}&85.1&72.3&48.3&58.1&73.7&72.9&  \\& \multirow{1}{*}{\centering PGD-100}&3.9&3.1&1.8&12.0&9.9&6.3&\underline{26.0}&\textbf{39.0}& \\
    \cmidrule(lr){1-1} \cmidrule(lr){2-2} 
    \cmidrule(lr){3-10}

\multirow{2}{*}{Places}&\multirow{1}{*}{\centering Clean}&\textbf{94.5}&92.3&94.8&73.1&55.7&75.0&83.3&\underline{93.0}&  \\& \multirow{1}{*}{\centering PGD-100}&4.9&3.7&4.7&12.7&12.1&14.1&\underline{41.7}&\textbf{68.3}& \\
    \cmidrule(lr){1-1} \cmidrule(lr){2-2} 
    \cmidrule(lr){3-10}

\multirow{2}{*}{LSUN}&\multirow{1}{*}{\centering Clean}&\underline{97.1}&91.6&96.6&76.0&55.6&83.1&89.2&\textbf{98.1}&  \\& \multirow{1}{*}{\centering PGD-100}&7.3&0.6&3.2&12.9&10.4&20.7&\underline{49.4}&\textbf{84.8}& \\
    \cmidrule(lr){1-1} \cmidrule(lr){2-2} 
    \cmidrule(lr){3-10}

\multirow{2}{*}{iSUN}&\multirow{1}{*}{\centering Clean}&\textbf{96.4}&91.4&96.4&72.5&54.8&80.1&86.5&\underline{95.1}&  \\& \multirow{1}{*}{\centering PGD-100}&7.5&0.9&3.1&11.9&10.6&22.1&\underline{47.3}&\textbf{77.3}& \\
    \cmidrule(lr){1-1} \cmidrule(lr){2-2} 
    \cmidrule(lr){3-10}

\multirow{2}{*}{Birds}&\multirow{1}{*}{\centering Clean}&96.6&\textbf{97.8}&95.1&73.1&54.5&78.4&93.4&\underline{96.8}&  \\& \multirow{1}{*}{\centering PGD-100}&7.4&10.5&14.2&13.4&11.0&23.7&\underline{66.2}&\textbf{75.9}& \\
    \cmidrule(lr){1-1} \cmidrule(lr){2-2} 
    \cmidrule(lr){3-10}

\multirow{2}{*}{Flower}&\multirow{1}{*}{\centering Clean}&96.8&96.6&98.9&77.6&69.6&85.1&\textbf{97.2}&\textbf{97.2}&  \\& \multirow{1}{*}{\centering PGD-100}&9.3&5.5&17.2&15.7&22.9&31.8&\textbf{80.1}&\underline{78.9}& \\
    \cmidrule(lr){1-1} \cmidrule(lr){2-2} 
    \cmidrule(lr){3-10}  

\multirow{2}{*}{COIL}&\multirow{1}{*}{\centering Clean}&\textbf{97.7}&\underline{88.1}&79.5&74.4&57.5&77.9&80.6&78.6&  \\& \multirow{1}{*}{\centering PGD-100}&15.7&3.5&0.8&16.3&14.0&19.2&\textbf{45.3}&\underline{44.8}& \\
    \cmidrule(lr){1-1} \cmidrule(lr){2-2} 
    \cmidrule(lr){3-10}  

\multirow{2}{*}{CIFAR10}&\multirow{1}{*}{\centering Clean}&\underline{92.9}&\textbf{94.8}&87.5&67.5&50.3&43.6&57.5&61.5  \\ & \multirow{1}{*}{\centering PGD-100}&9.1&5.8&3.7&10.7&10.3&3.0&\underline{13.8}&\textbf{30.7}  \\
\cmidrule(lr){1-1} \cmidrule(lr){2-2} 
\cmidrule(lr){3-9}  

\noalign{\smallskip}
\multirow{2}{*}{Avg.}&\multirow{1}{*}{\centering Clean}&\textbf{95.8}&\underline{91.5}&91.6&70.0& 61.5 &79.3&87.7&88.1&   \\& \multirow{1}{*}{\centering PGD-100}&8.8&3.7&5.4&13.6&21.6&26.4&\underline{55.3}&\textbf{66.4}  \\
 \hline
\end{tabular}}
\end{subtable}
 
\end{table*}

\input{Samples/Samples}
